# Supplementary material for: Group-wise normalization in differential abundance analysis of microbiome samples
Source: arXiv:2411.15400 source file (2024-11-23)
Supplement: Supplementary file 1 [file Supplementary_materials.pdf]

# Supplementary Materials to “Group-wise normalization in differential abundance analysis of microbiome samples”

## 1 Justification of bias correction

In this section, we expand on the mathematical heuristic presented in the main text by showing that the proposed group-wise normalization methods can counter-act the compositional bias term we defined previously. The model we consider for the taxon counts is

$$\begin{aligned}\log(A_{ij}) &= \beta_{0j} + \beta_{1j}X_i \\ R_{ij} &= \frac{A_{ij}}{\sum_{j=1}^q A_{ij}} \\ S_i &\stackrel{\text{iid}}{\sim} \mathcal{D} \\ \mathbf{Y}_i &= (Y_{i1}, \dots, Y_{iq})^T \stackrel{\text{iid}}{\sim} \text{Multinomial}(S_i, \mathbf{R}_i),\end{aligned}$$

$i \in \{1, \dots, n\}$ ,  $j \in \{1, \dots, q\}$ . Here,  $X_i \in \{0, 1\}$  denotes group membership of sample  $i$ ,  $\mathbf{Y}_i = (Y_{i1}, \dots, Y_{iq})^T$  are the observed taxon counts,  $\mathbf{R}_i = (R_{i1}, \dots, R_{iq})^T$  are the unknown true relative abundances of those samples, and  $\mathbf{A}_i = (A_{i1}, \dots, A_{iq})^T$  are the unknown absolute abundances. The library sizes  $S_i$  follow an arbitrary distribution  $\mathcal{D}$  with finite mean and variance. The main parameter of interest is  $\beta_{1j}$ , the true log fold change in absolute abundance.

For convenience, for  $g \in \{0, 1\}$ , let

$$R_j^{(g)} = \frac{\beta_{0j} + \beta_{1j}g}{\sum_{k=1}^q \beta_{0k} + \beta_{1k}g}$$

be the group-level relative abundance of taxon  $j$  in group  $g$ . Since there is no noise term in the definition of  $\log(A_{ij})$ , we have that  $R_{ij} = R_j^{(g)}$  for all  $j$  and  $i$  such that  $X_i = g$ . In other words, the true relative abundance of a given sample equals the group-level relative abundance of its group.

A Poisson model for this data would take the form

$$\begin{aligned}\log(\lambda_{ij}) &= \alpha_{0j} + \alpha_{1j}X_i + \log(\psi_i) \\ Y_{ij} &\sim \text{Poisson}(\lambda_{ij}),\end{aligned}$$

where  $\psi_i$  is the specified offset, such as the normalization factor. The maximum likelihood estimator for  $\alpha_{1j}$  is then

$$\hat{\alpha}_{1j} = \log\left(\frac{\sum_{i=1}^n Y_{ij}X_i / \sum_{i=1}^n Y_{ij}(1-X_i)}{\sum_{i=1}^n \psi_i X_i / \sum_{i=1}^n \psi_i (1-X_i)}\right).$$

In total sum scaling (TSS) normalization, the offset term is set to be  $S_i$  and the estimator becomes

$$\hat{\alpha}_{1j}^{\text{TSS}} = \log\left(\frac{\hat{R}_j^{(1)}}{\hat{R}_j^{(0)}}\right),$$

where,

$$\hat{R}_j^{(g)} = \frac{\sum_{i=1}^n Y_{ij} \mathbb{1}(X_i = g)}{\sum_{i=1}^n S_i \mathbb{1}(X_i = g)}$$

is the estimated relative abundance of group  $g$ ,  $g \in \{0, 1\}$ . Since  $\hat{\alpha}_{1j}^{\text{TSS}}$  is the log ratio of  $\hat{R}_j^{(1)}$  to  $\hat{R}_j^{(0)}$ , we will refer to  $\alpha_{1j}^{\text{TSS}}$  as the observed LFC of taxon  $j$ ,  $j \in \{1, \dots, q\}$ .

Now, since  $Y_{1j}, \dots, Y_{nj}$  are i.i.d with mean  $\mathbb{E}[S_1]R_j^{(g)}$  and finite variance, we know

$$\begin{aligned}\hat{R}_j^{(g)} &= \frac{\sum_{i=1}^n Y_{ij} \mathbb{1}(X_i = g)}{\sum_{i=1}^n S_i \mathbb{1}(X_i = g)} \\ &= \frac{\frac{1}{n} \sum_{i=1}^n Y_{ij} \mathbb{1}(X_i = g)}{\frac{1}{n} \sum_{i=1}^n S_i \mathbb{1}(X_i = g)} \\ &\xrightarrow{p} \frac{\mathbb{E}[S_1]R_j^{(g)}}{\mathbb{E}[S_1]} = R_j^{(g)}\end{aligned}$$

as  $n \rightarrow \infty$  by the weak law of large numbers and the continuous mapping theorem,  $g \in 0, 1$ ,  $j \in \{1, \dots, q\}$ . As second application of the continuous mapping theorem yields

$$\begin{aligned}\hat{\alpha}_{1j}^{\text{TSS}} &\xrightarrow{p} \log(R_j^{(1)}) - \log(R_j^{(0)}) \\ &= \log\left(\frac{\beta_{0j} + \beta_{1j}}{\sum_{k=1}^q \beta_{0k} + \beta_{1k}}\right) - \log\left(\frac{\beta_{0j}}{\sum_{k=1}^q \beta_{0k}}\right) \\ &= \beta_{1j} + \log\left(\frac{\sum_{k=1}^q \beta_{0k}}{\sum_{k=1}^q \beta_{0k} + \beta_{1k}}\right) \\ &= \beta_{1j} + \Delta,\end{aligned}$$

where  $\Delta$  denotes the compositional bias. We demonstrate how the proposed normalization counteracts this bias in the next two subsections.

## 1.1 G-RLE

In G-RLE normalization, the offset term for sample  $i$  is set as

$$\psi_i = S_i \times C_j^{(X_i)},$$

where

$$C_j^{(X_i)} = \text{median}_j \left( \sqrt{\frac{\hat{R}_j^{(X_i)}}{\hat{R}_j^{(1-X_i)}}} \right).$$

Thus we have

$$\begin{aligned}\hat{\alpha}_j^{\text{G-RLE}} &= \log\left(\frac{\sum_{j=1}^q Y_{ij} X_i}{C_j^{(1)} \sum_{j=1}^q S_i X_i} / \frac{\sum_{j=1}^q Y_{ij} (1 - X_i)}{C_j^{(0)} \sum_{j=1}^q S_i (1 - X_i)}\right) \\ &= \hat{\alpha}_j^{\text{TSS}} - \log\left(\frac{C_j^{(1)}}{C_j^{(0)}}\right).\end{aligned}$$

The new component  $\log(C_j^{(1)}/C_j^{(0)})$  performs bias correction. To see this, assume  $\text{median}_j(\beta_{1j}) = 0$  and notice that

$$\begin{aligned}\log\left(\frac{C_j^{(1)}}{C_j^{(0)}}\right) &= \log(C_j^{(1)}) - \log(C_j^{(0)}) \\ &= \frac{1}{2} \text{median}_j \left( \log\left(\frac{\hat{R}_j^{(1)}}{\hat{R}_j^{(0)}}\right) \right) - \frac{1}{2} \text{median}_j \left( \log\left(\frac{\hat{R}_j^{(0)}}{\hat{R}_j^{(1)}}\right) \right) \\ &= \text{median}_j \left( \log\left(\frac{\hat{R}_j^{(1)}}{\hat{R}_j^{(0)}}\right) \right) \\ &\xrightarrow{p} \text{median}_j \left( \beta_{1j} + \Delta \right) \\ &= \text{median}_j \left( \beta_{1j} \right) + \Delta \\ &= \Delta.\end{aligned}$$

Altogether,  $\hat{\alpha}_{1j}^{\text{G-RLE}} \xrightarrow{p} \beta_{1j} + \Delta - \Delta = \beta_{1j}$ .

## 1.2 FTSS

In FTSS normalization, we restrict the library size to include only taxa whose observed log fold changes ( $\hat{\alpha}_{1j}^{\text{TSS}}$ ) falls within  $100 \times \frac{p^*}{2}$  percentiles of the mode. To understand why this works, assume  $\text{mode}_j(\beta_{1j}) = 0$  and  $\sum_{j=1}^q \mathbb{1}(\beta_{1j} = 0) > \lceil qp^* \rceil$ , where  $\lceil \cdot \rceil$  denotes the ceiling function, and let  $Q = \{j : \beta_{1j} = 0\}$ . Since  $\hat{\alpha}_{1j}^{\text{TSS}} \xrightarrow{p} \Delta + \beta_{1j}$  for all  $j$ , we have, for any  $\epsilon \in (0, \min_{j \notin Q} |\beta_{1j}|)$ ,

$$P\left(\max_{j \in Q} |\hat{\alpha}_{1j}^{\text{TSS}} - \Delta| > \epsilon\right) \rightarrow 0$$

and

$$P\left(\min_{j \notin Q} |\hat{\alpha}_{1j}^{\text{TSS}} - \Delta| > \epsilon\right) \rightarrow 1$$

as  $n \rightarrow \infty$ . These together imply

$$P\left(\max_{j \in Q} |\hat{\alpha}_{1j}^{\text{TSS}} - \Delta| < \min_{j \notin Q} |\hat{\alpha}_{1j}^{\text{TSS}} - \Delta|\right) \rightarrow 1.$$

Thus, with probability converging to 1, there is an interval around  $\Delta$  containing all the observed log fold changes of equally abundant taxa no observed log fold changes of differentially abundant taxa. We use this to define reference taxa by estimating  $\Delta$  as  $\hat{\Delta} = \text{mode}_j(\hat{\alpha}_{1j}^{\text{TSS}})$ , then choosing the  $\lfloor \frac{p^* q}{2} \rfloor$  log fold changes below and above  $\hat{\Delta}$ . Since, as assumed, at least  $\lceil p^* q \rceil$  taxa are equally abundant, we should expect to get mostly taxa with  $\beta_{1j}$  either zero or close to zero.

What we must justify now is that a proper choice of reference taxa will eliminate the compositional bias. To see this, let  $W \subseteq Q$  and  $S_i^W = \sum_{j \in W} Y_{ij}$ ,  $j \in W$ . We must show that setting  $\psi_i = S_i^W$  corrects our estimator. Indeed, we have

$$\begin{aligned} \hat{\alpha}_{1j}^W &= \log\left(\frac{\sum_{i=1}^n Y_{ij} X_i}{\sum_{i=1}^n S_i^W X_i} / \frac{\sum_{i=1}^n Y_{ij} (1 - X_i)}{\sum_{i=1}^n S_i^W (1 - X_i)}\right) \\ &= \log\left(\frac{\frac{1}{n} \sum_{i=1}^n Y_{ij} X_i}{\frac{1}{n} \sum_{i=1}^n S_i^W X_i} / \frac{\frac{1}{n} \sum_{i=1}^n Y_{ij} (1 - X_i)}{\frac{1}{n} \sum_{i=1}^n S_i^W (1 - X_i)}\right) \\ &\rightarrow \log\left(\frac{R_j^{(1)}}{R_j^{(0)}}\right) - \log\left(\frac{\mathbb{E}[S_i^W | X_i = 1]}{\mathbb{E}[S_i^W | X_i = 0]}\right) \\ &= \beta_{1j} + \Delta - \log\left(\frac{\mathbb{E}[S_i^W | X_i = 1]}{\mathbb{E}[S_i^W | X_i = 0]}\right). \end{aligned}$$

Now notice that

$$\begin{aligned} \mathbb{E}[S_i^W | X_i = 1] &= \mathbb{E}[S_1] \sum_{j \in Q}^q R_j^{(1)} \\ &= \mathbb{E}[S_1] \frac{1}{\sum_{k=1}^q \beta_{0k} + \beta_{1k}} \sum_{j \in Q} \beta_{0j} \end{aligned}$$

and, similarly,

$$\mathbb{E}[S_i^W | X_i = 0] = \mathbb{E}[S_1] \frac{1}{\sum_{k=1}^q \beta_{0k}} \sum_{j \in Q} \beta_{0j}.$$

Taking the log ratio of these gives us that

$$\log\left(\frac{\mathbb{E}[S_i^W | X_i = 1]}{\mathbb{E}[S_i^W | X_i = 0]}\right) = \log\left(\frac{\sum_{k=1}^q \beta_{0k}}{\sum_{k=1}^q \beta_{0k} + \beta_{1k}}\right) = \Delta.$$

Thus,  $\hat{\alpha}_{1j}^W \rightarrow \beta_{1j}$ , as desired.

## 2 Differential abundance analysis methods

**Table S1:** Normalization-based differential abundance analysis methods

| Method                               | Implementation                                                             | Model Summary                                          |
|--------------------------------------|----------------------------------------------------------------------------|--------------------------------------------------------|
| edgeR [Robinson et al., 2010]        | <code>exactTest</code> function from <code>edgeR</code> R package          | Negative binomial model                                |
| DESeq2 [Love et al., 2014]           | <code>DESeq</code> function from <code>DESeq2</code> R package             | Negative binomial model with empirical Bayes shrinkage |
| MetagenomeSeq [Paulson et al., 2013] | <code>fitFeature</code> function from <code>metagenomeSeq</code> R package | Zero-inflated log-normal model                         |

## 3 Confounder-adjusted simulations

In this section, we describe an extension of the model-based simulations in which the analysis adjusts for a single confounding variable. As in the main text simulations, we compared the performance of FTSS and G-RLE to the existing normalization methods TSS, TMM, RLE, GMPR, CSS, and Wrench, paired with the DAA methods edgeR and DESeq2. The DAA method MetagenomeSeq is not included since it does not allow covariates. We evaluated the methods in terms of their observed true positive rate (TPR) and false discovery rate (FDR) at a nominal FDR level of 0.05. We averaged these values over 1,000 replicates of each of 18 different settings, described below.

### 3.1 Data generation and settings

We simulated data from the hierarchical multinomial model described in the main text, but with the addition of a continuous confounding variable  $U_i$ ,  $i \in \{1, \dots, n\}$ . Specifically, we generated the absolute ( $B_{ij}$ ) and relative ( $B'_{ij}$ ) abundances as:

$$\begin{aligned}
\mathbf{V}_i &= (V_{i1}, \dots, V_{iq})^T \sim \text{MVN}(\mathbf{0}, \sigma^2 \Sigma_v) \\
U_i &\sim \text{N}(X_i, 1) \\
\log(A_{ij}) &= \beta_{0j} + \beta_{1j} X_i + \theta_j U_i + V_{ij} \\
\mathbf{Z}_i &= (Z_{i1}, \dots, Z_{iq})^T \sim \text{MVN}(\mathbf{0}, \Sigma_z) \\
B_{ij} &= A_{ij} \mathbb{1}(Z_{ij} > \alpha) \\
B'_{ij} &= \frac{B_{ij}}{\sum_{j=1}^q B_{ij}},
\end{aligned}$$

$i \in \{1, \dots, n\}$ ,  $j \in \{1, \dots, q\}$ . The latent variables  $V_{ij}$  add variance in the absolute abundances as well as correlation between taxa. The overall degree of variance is governed by the parameter  $\sigma^2$ , and the correlations are governed by the correlation matrix  $\Sigma_v$ . The parameter  $\beta_{1j}$  is the group-level log fold change (LFC) of interest, and the parameter  $\theta_j$  is the LFC associated with a one-unit change in the confounding variable  $U_i$ . Finally, the latent variables  $Z_{ij}$  introduce zero-inflation; the correlation between zeros is controlled by  $\Sigma_z$ , a correlation matrix, and the overall degree of zero-inflation is controlled by the parameter  $\alpha$ . Now, letting  $\mathbf{B}'_i = (B'_{i1}, \dots, B'_{iq})^T$ , we sampled the final taxon counts as:

$$\begin{aligned}
S_i &\sim \text{Negative Binomial}(\mu_S, \gamma_S^2) \\
\mathbf{Y}_i &= (Y_{i1}, \dots, Y_{iq})^T \sim \text{Multinomial}(S_i, \mathbf{B}'_i),
\end{aligned}$$

where  $\mu_S$  and  $\gamma_S^2$  are the mean and variance of the negative binomial distribution, respectively, and  $S_i$  is the library size.

The parameters  $\Sigma_v$ ,  $\Sigma_z$ ,  $\alpha$ ,  $\beta_{0j}$ ,  $\mu_S$ , and  $\gamma_S^2$  are fixed across all settings to their same values from the main text. The sample size  $n$  is set to 200 or 500, half with  $X_i = 0$  and half with  $X_i = 1$ . The parameter  $\sigma^2$  is set as 1, 1.5, or 2, which we denote as low, medium, or high variance settings, respectively. The parameter  $\boldsymbol{\beta}_1 = (\beta_{1j}, \dots, \beta_{1q})$  is determined by setting every entry to zero except the first 10%, 20%, or 30%, which are sampled from a  $\text{N}(1, 1)$  distribution. Finally, the confounding effects  $\theta_j$ ,  $j \in 1, \dots, q$ , are chosen by setting  $\theta_j = \beta_{1j}/2$  if  $\beta_{1j} \neq 0$ , and  $\theta_j \sim \text{N}(0, 0.5)$  otherwise. This ensures the confounding variable has some effect on every taxa, and that the direction of the confounder effect is the same as the direction of the group effect, if there is one.

### 3.2 Confounder-adjusted Simulation Results

Results for the confounder-adjusted simulations are presented in the next two pages.

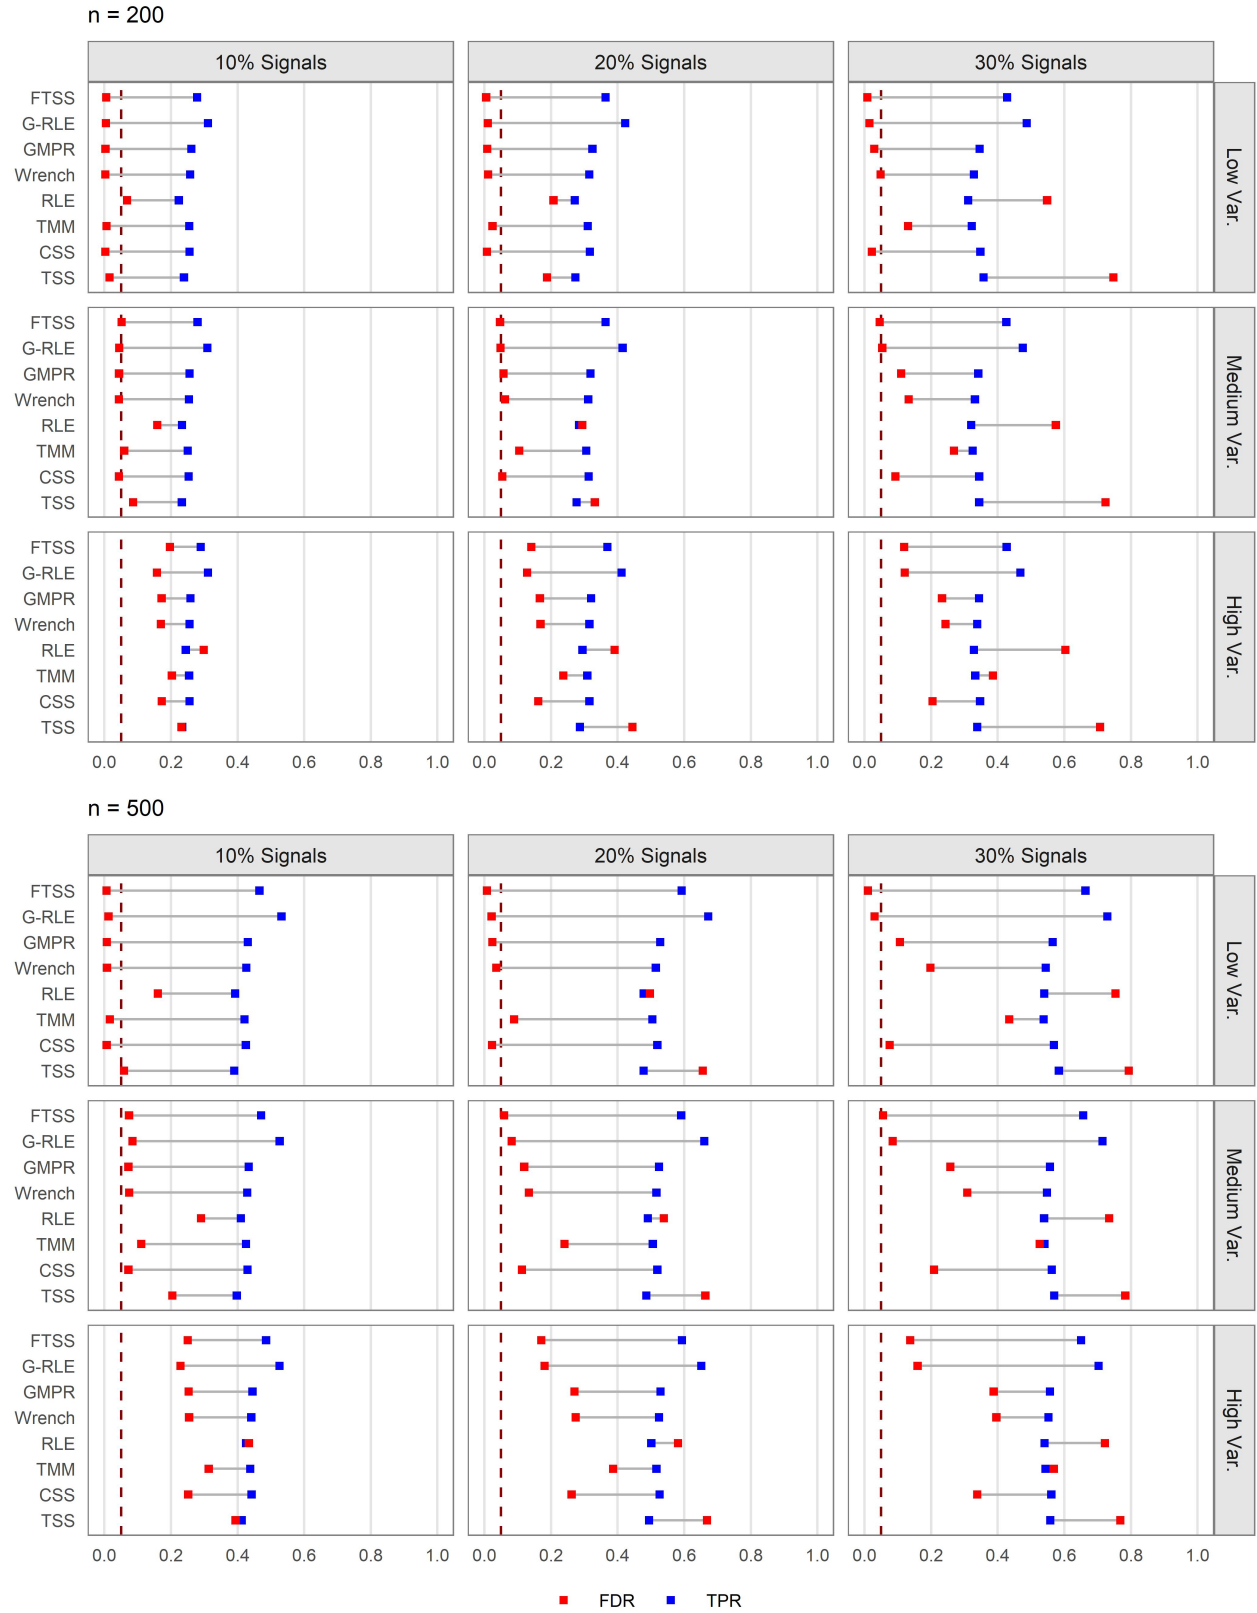

**Figure S1: Performance of normalization methods at nominal false discovery rate in model-based simulations with the DAA methods edgeR, adjusting for a confounding variable.** The true positive rate (blue) and observed false discovery rate (red) corresponding to a nominal false discovery rate of 0.05 (the dashed line). Value shown is the mean over 1,000 replicates of each setting. The simulated datasets contain 300 taxa and either 200 or 500 samples. Either 10%, 20% or 30% of the taxa are differentially abundant, with log fold changes sampled from a Normal(1,1) distribution. Three different variance settings are considered.

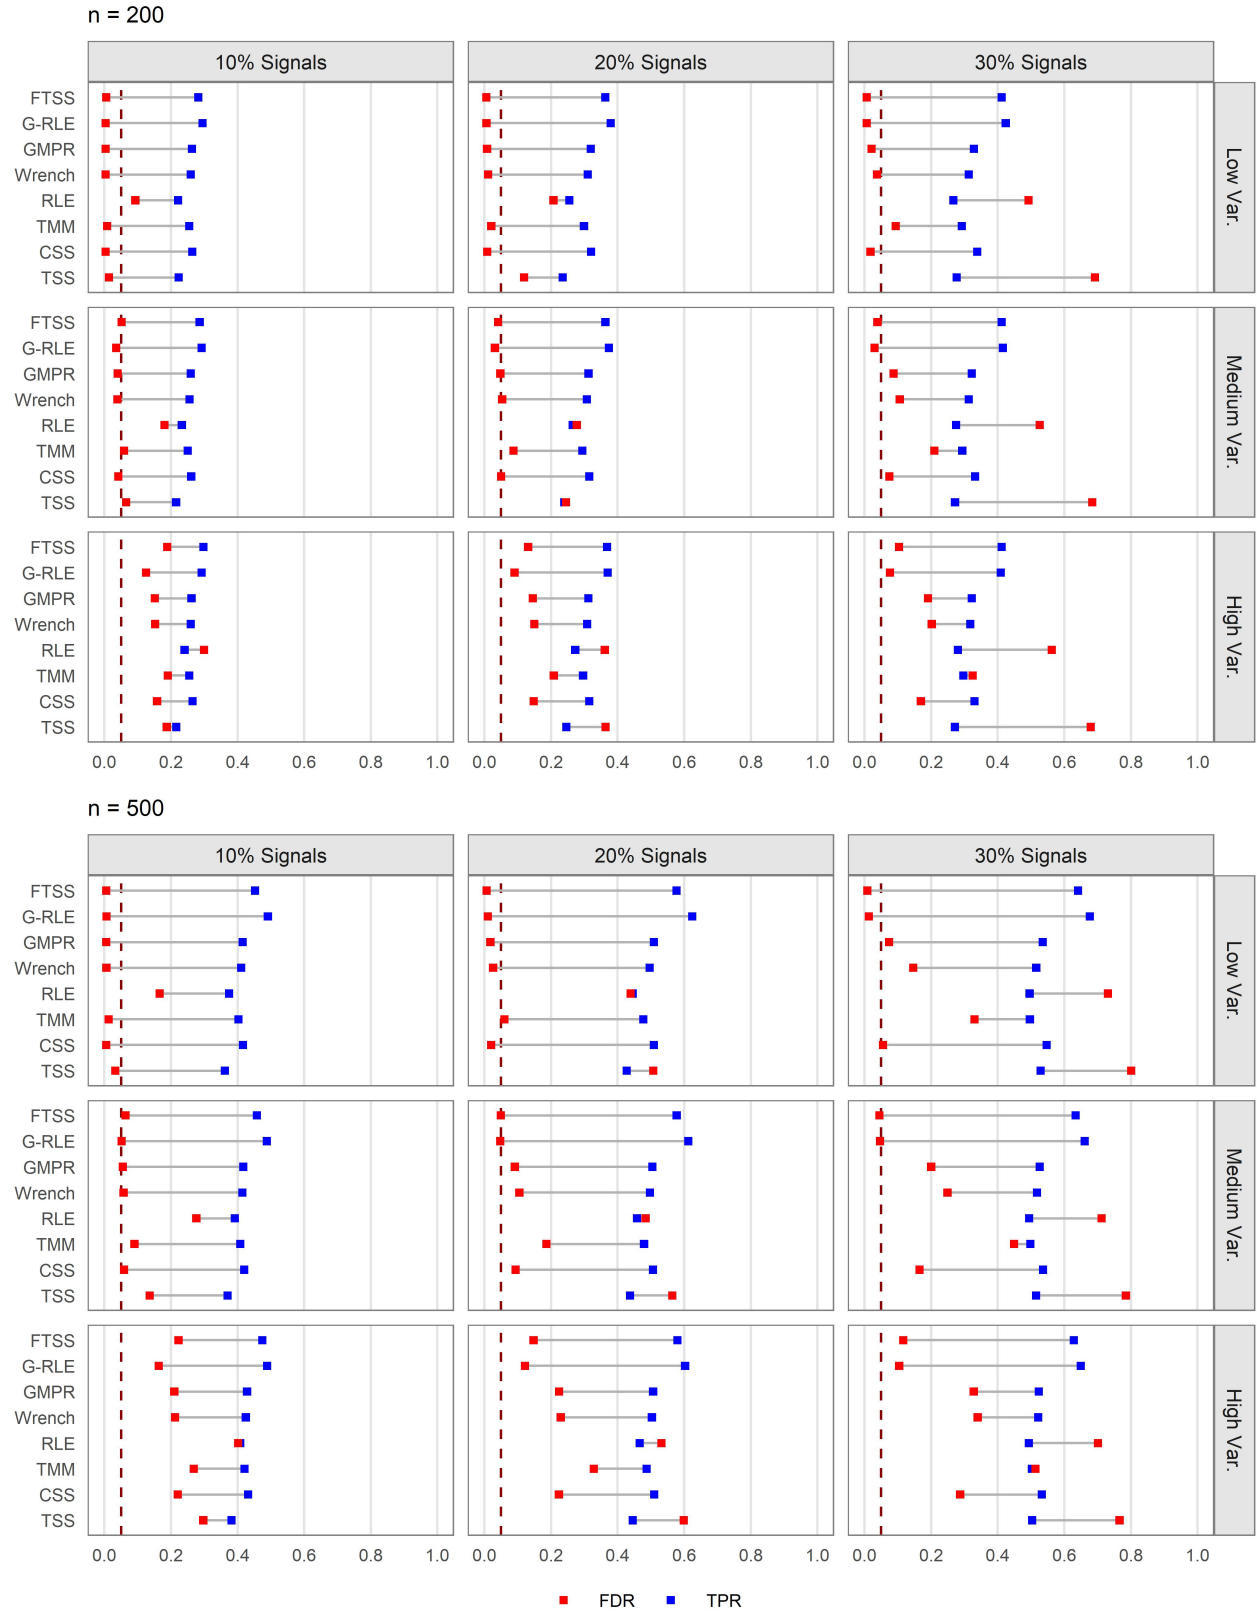

**Figure S2: Performance of normalization methods at nominal false discovery rate in model-based simulations with the DAA methods DESeq2, adjusting for a confounding variable.** The true positive rate (blue) and observed false discovery rate (red) corresponding to a nominal false discovery rate of 0.05 (the dashed line). Value shown is the mean over 1,000 replicates of each setting. The simulated datasets contain 300 taxa and either 200 or 500 samples. Either 10%, 20% or 30% of the taxa are differentially abundant, with log fold changes sampled from a Normal(1,1) distribution. Three different variance settings are considered.

## 4 Complete results for main text simulations

### 4.1 TPR by FPR Curves

In this section, we present the true positive rate (TPR) by false positive rate (FPR) curves for every normalization, differential abundance analysis (DAA) method, and simulation setting described in the main text.

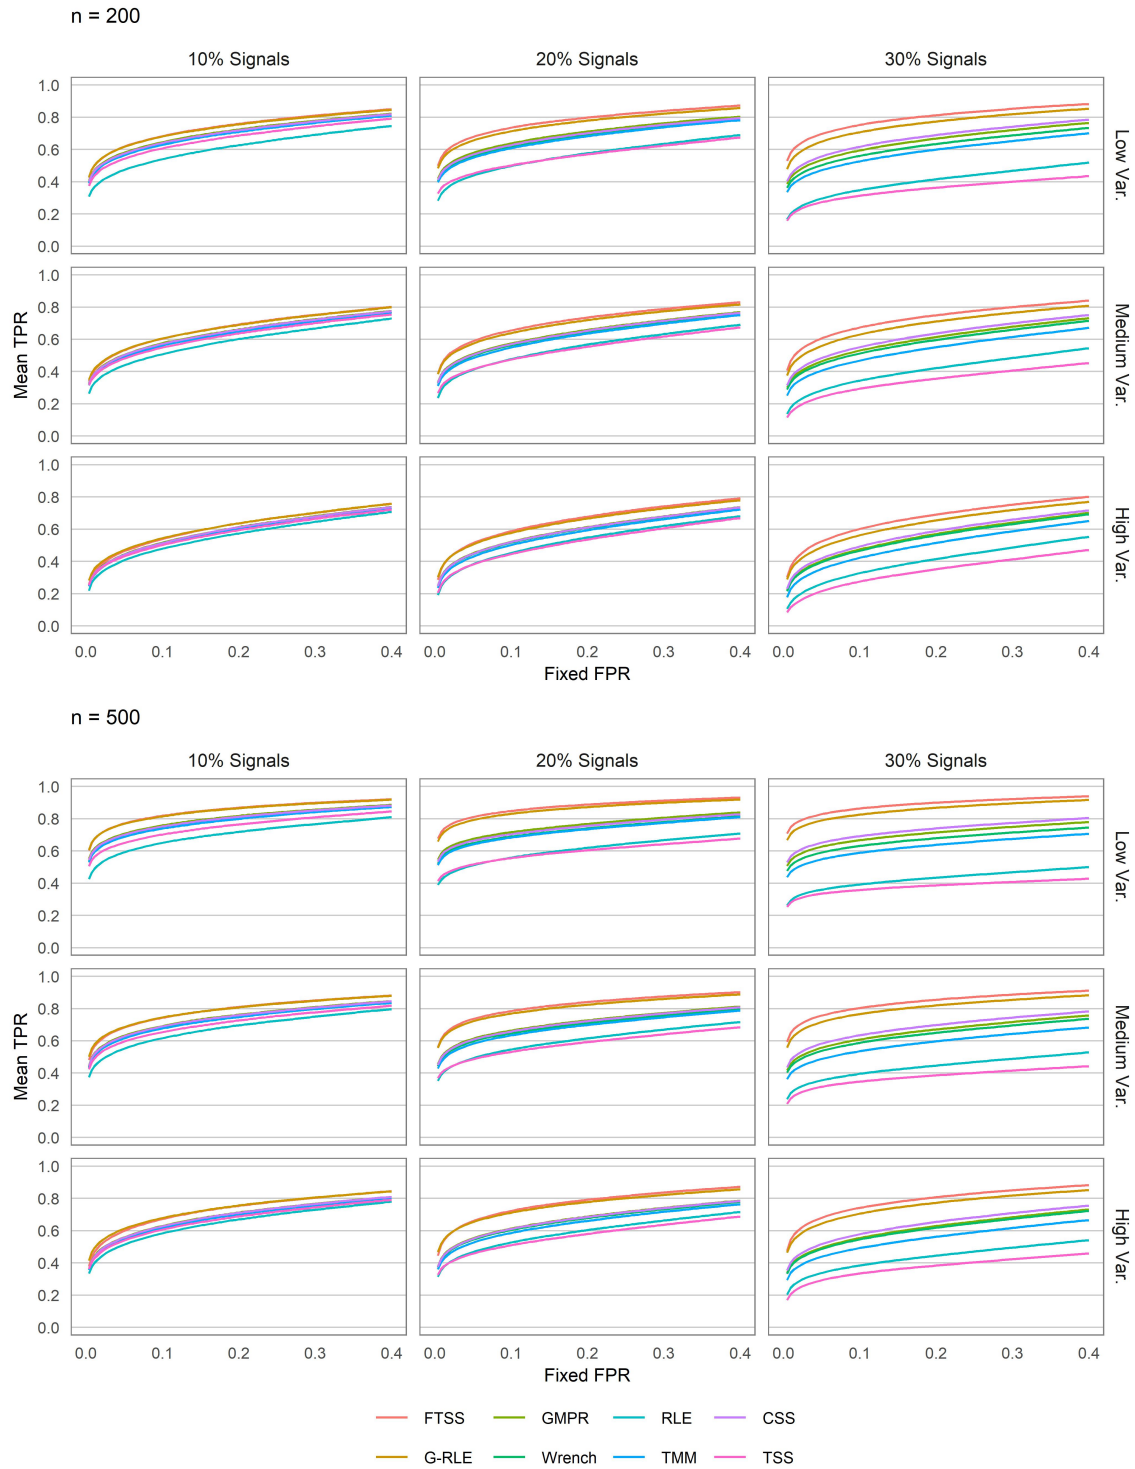

**Figure S3: True positive rate for detecting differentially abundant taxa in model-based simulations with the DAA method edgeR.** The true positive rate for detecting differentially abundant taxa at fixed values of the false positive rate. Value shown is the mean over 1,000 replicates of each setting. The simulated datasets contain 300 taxa and either 200 or 500 samples. Either 10%, 20% or 30% of the taxa are differentially abundant, with log fold changes sampled from a Normal(1,1) distribution. Three different variance settings are considered.

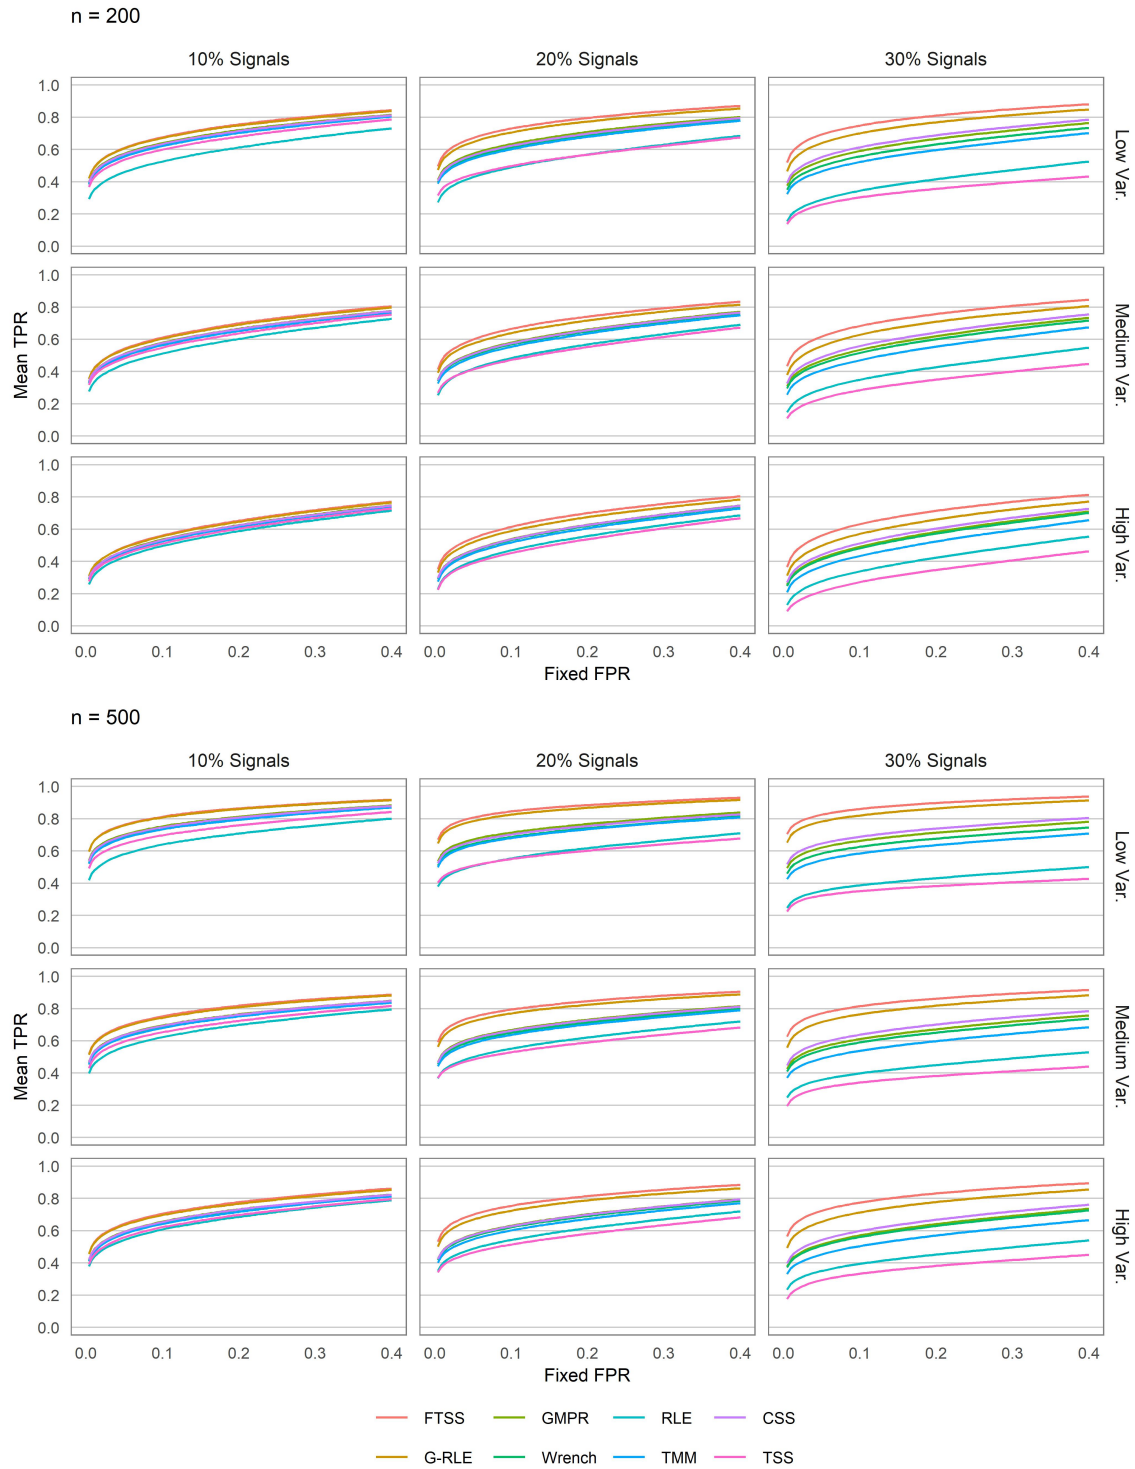

**Figure S4: True positive rate for detecting differentially abundant taxa in model-based simulations with the DAA method DESeq2.** The true positive rate for detecting differentially abundant taxa at fixed values of the false positive rate. Value shown is the mean over 1,000 replicates of each setting. The simulated datasets contain 300 taxa and either 200 or 500 samples. Either 10%, 20% or 30% of the taxa are differentially abundant, with log fold changes sampled from a Normal(1,1) distribution. Three different variance settings are considered.

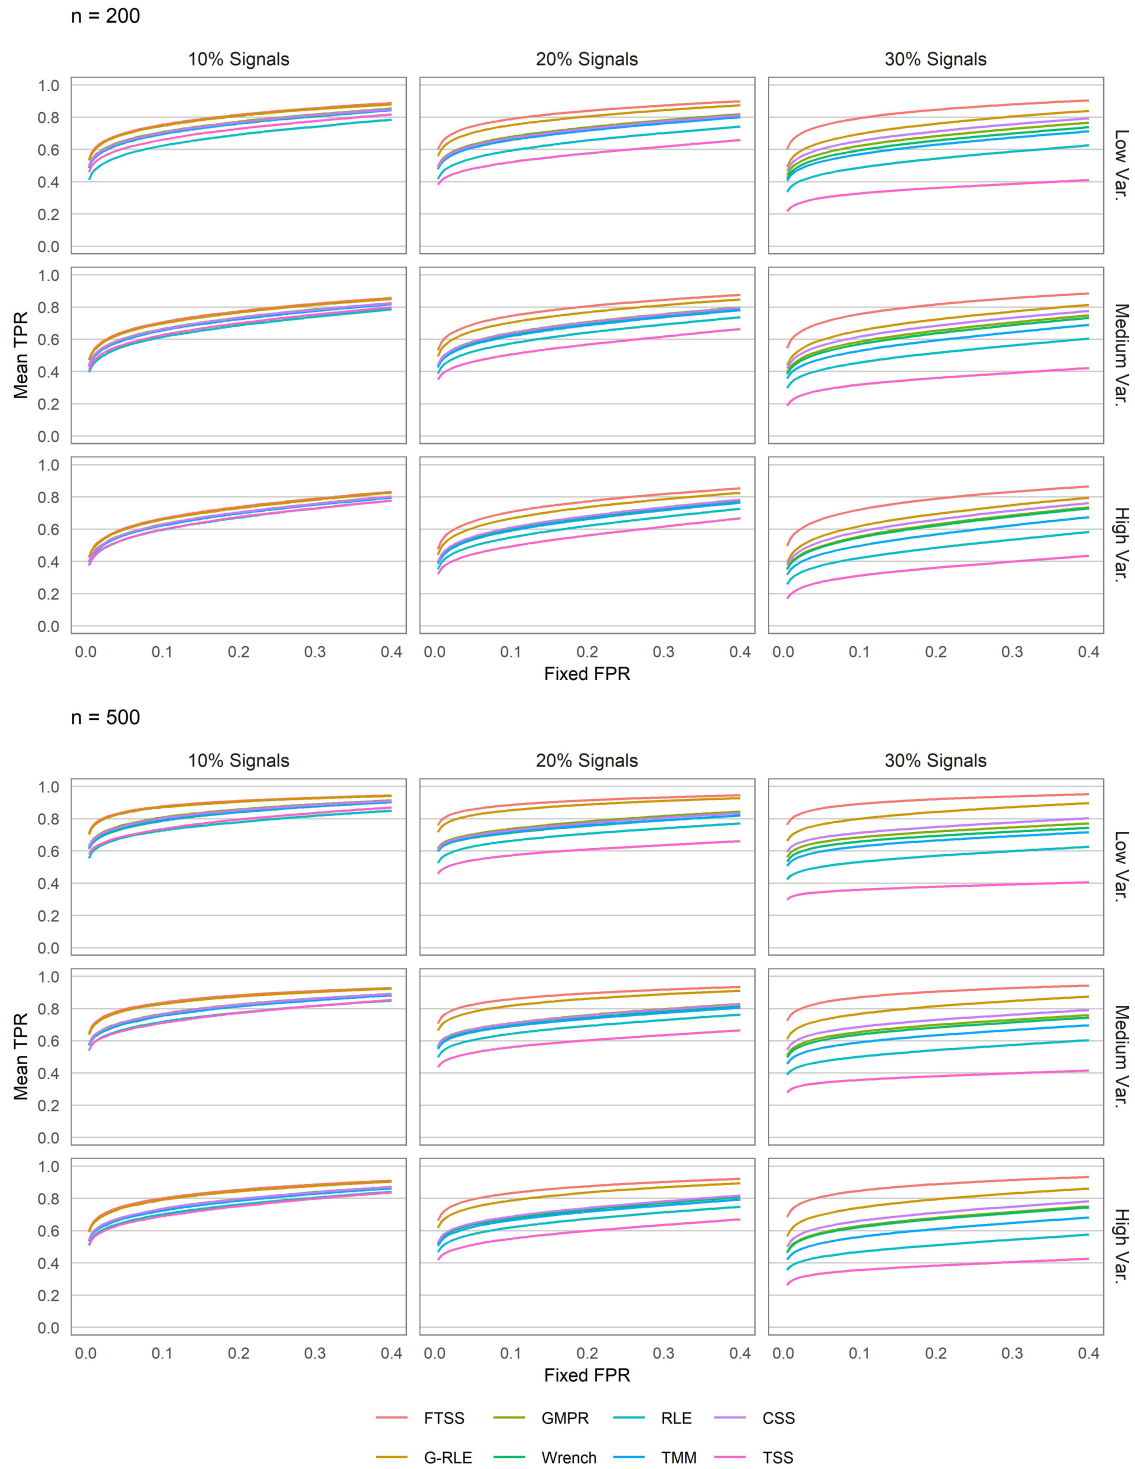

**Figure S5: True positive rate for detecting differentially abundant taxa in model-based simulations with the DAA method MetagenomeSeq.** The true positive rate for detecting differentially abundant taxa at fixed values of the false positive rate. Value shown is the mean over 1,000 replicates of each setting. The simulated datasets contain 300 taxa and either 200 or 500 samples. Either 10%, 20% or 30% of the taxa are differentially abundant, with log fold changes sampled from a Normal(1,1) distribution. Three different variance settings are considered.

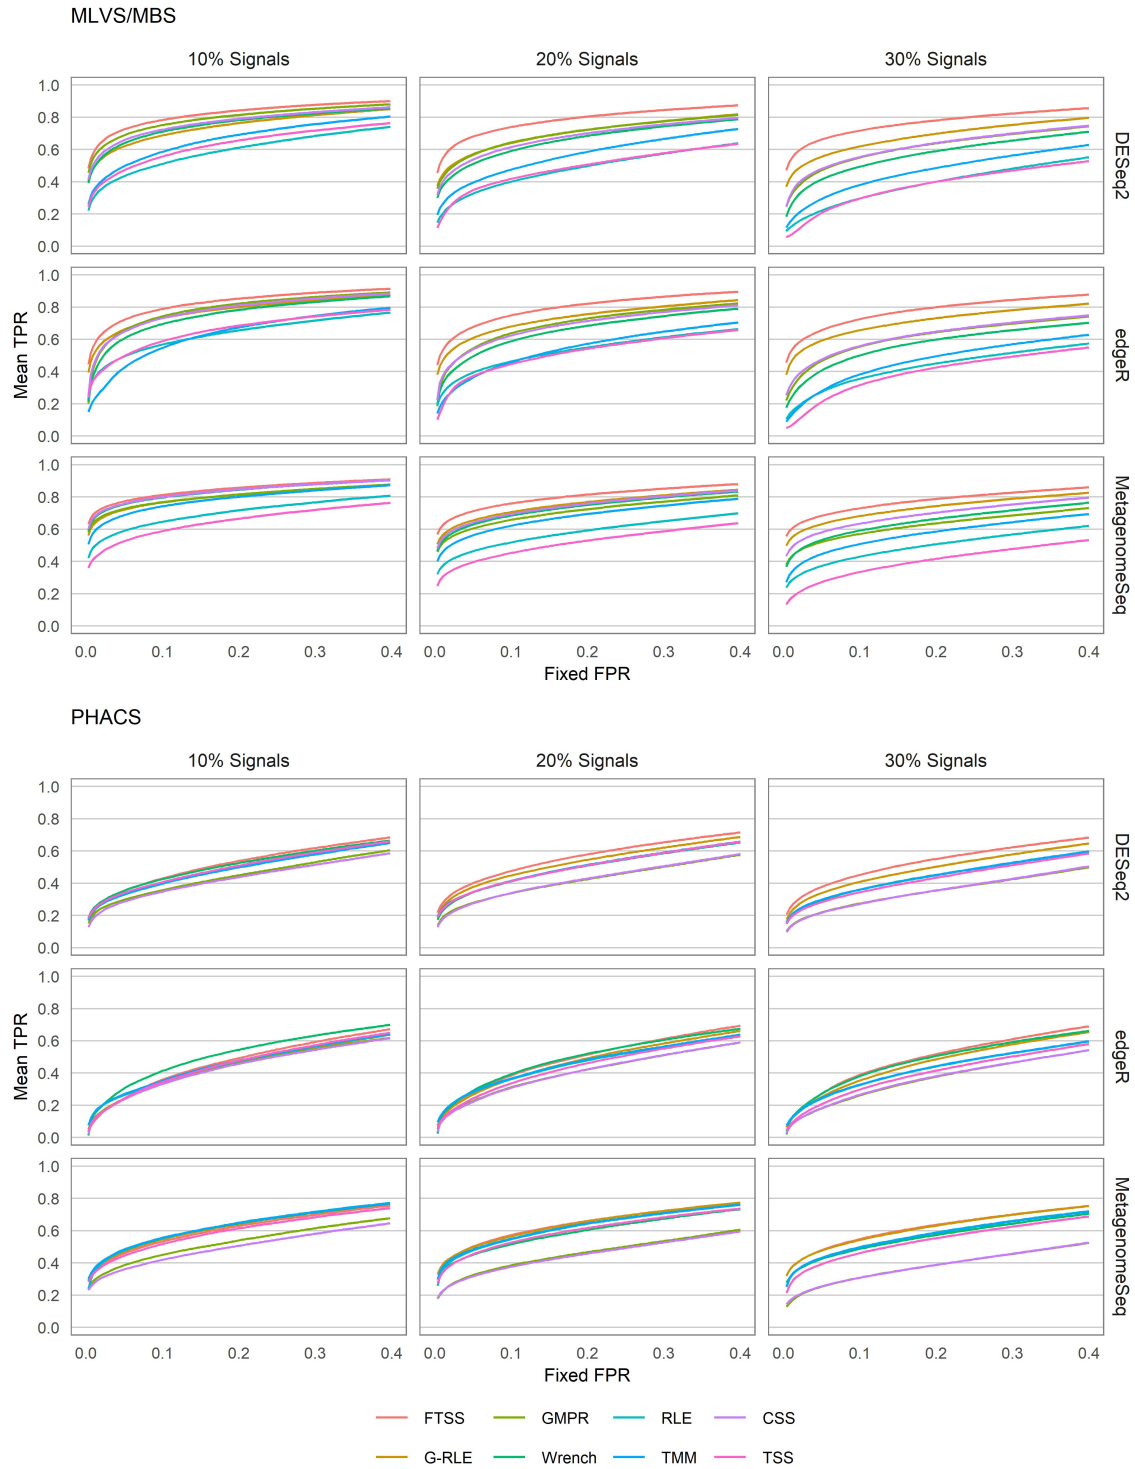

**Figure S6: True positive rate for testing differentially abundant taxa in synthetic data simulations.** The true positive rate for detecting differentially abundant taxa at fixed values of the false positive rate, for synthetic microbiome data based on either the MLVS/MBS or PHACS data. Value shown is the mean over 1,000 replicates of each setting. Either 10%, 20% or 30% of the taxa are simulated to be differentially abundant, with log fold changes sampled from a Normal(1,1) distribution.

## 4.2 Performance at 5% nominal FDR

In this section, we present the average observed true positive rate (TPR) and false discovery rate (FDR) at a nominal FDR level of 0.05, for every normalization, differential abundance analysis (DAA) method, and simulation setting described in the main text.

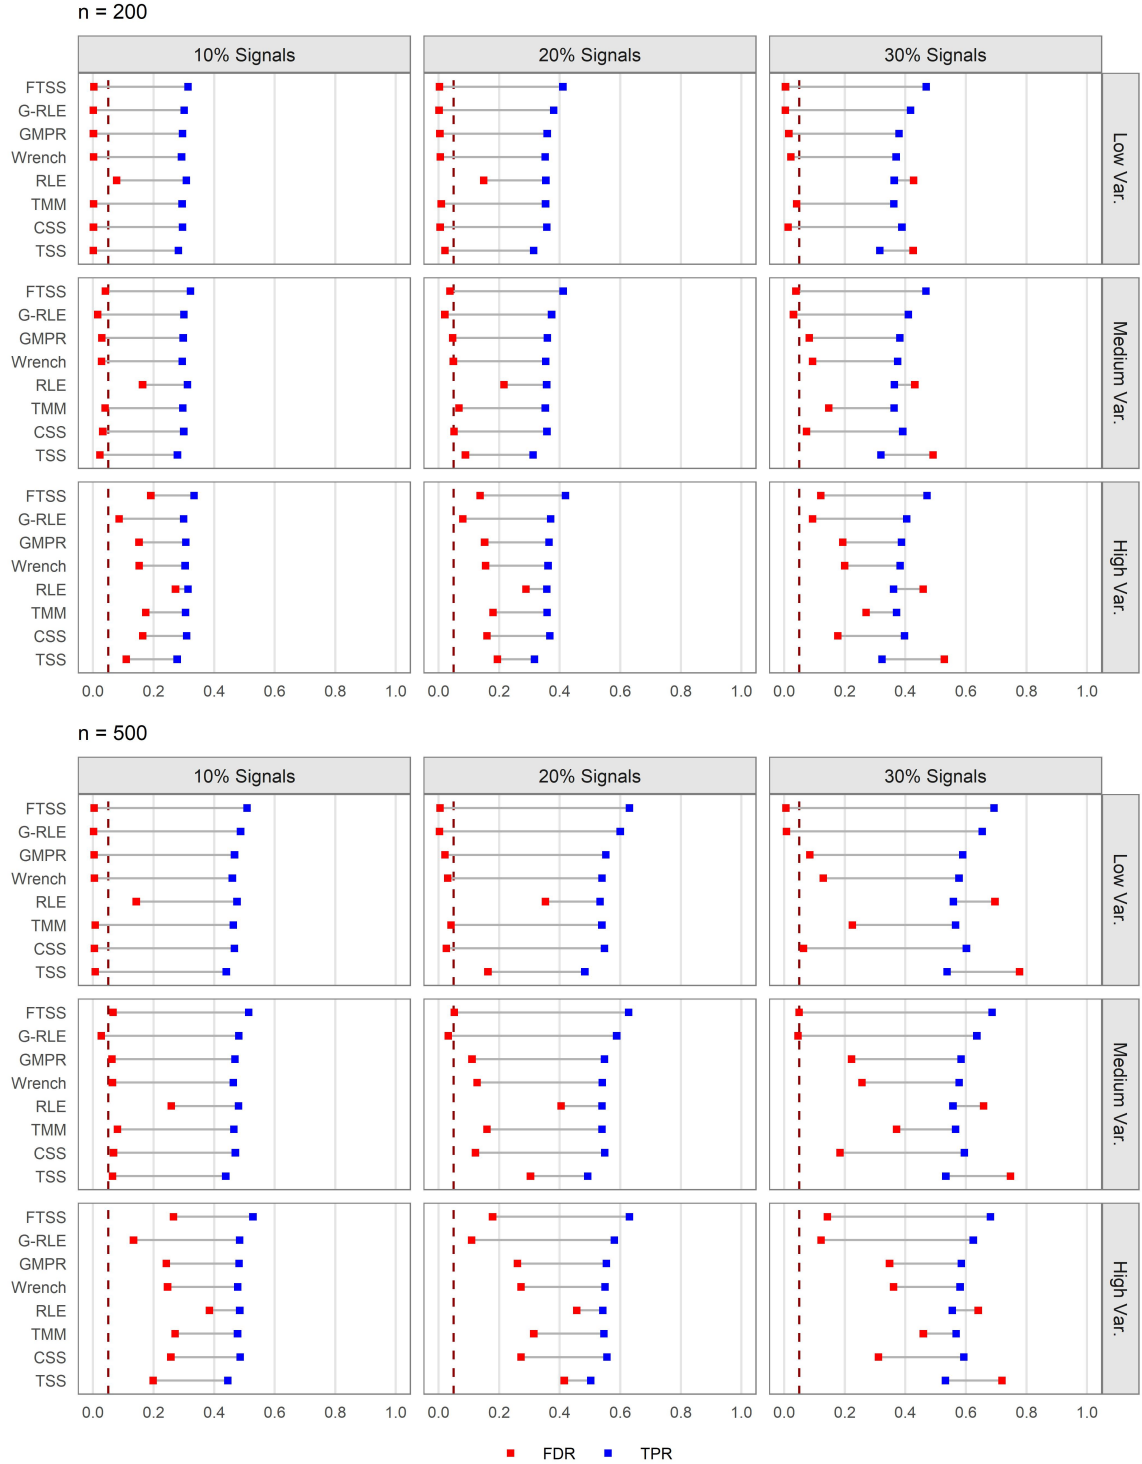

**Figure S7: Performance of normalization methods at nominal false discovery rate in model-based simulations with the DAA methods edgeR.** The true positive rate (blue) and observed false discovery rate (red) corresponding to a nominal false discovery rate of 0.05 (the dashed line). Value shown is the mean over 1,000 replicates of each setting. The simulated datasets contain 300 taxa and either 200 or 500 samples. Either 10%, 20% or 30% of the taxa are differentially abundant, with log fold changes sampled from a Normal(1,1) distribution. Three different variance settings are considered.

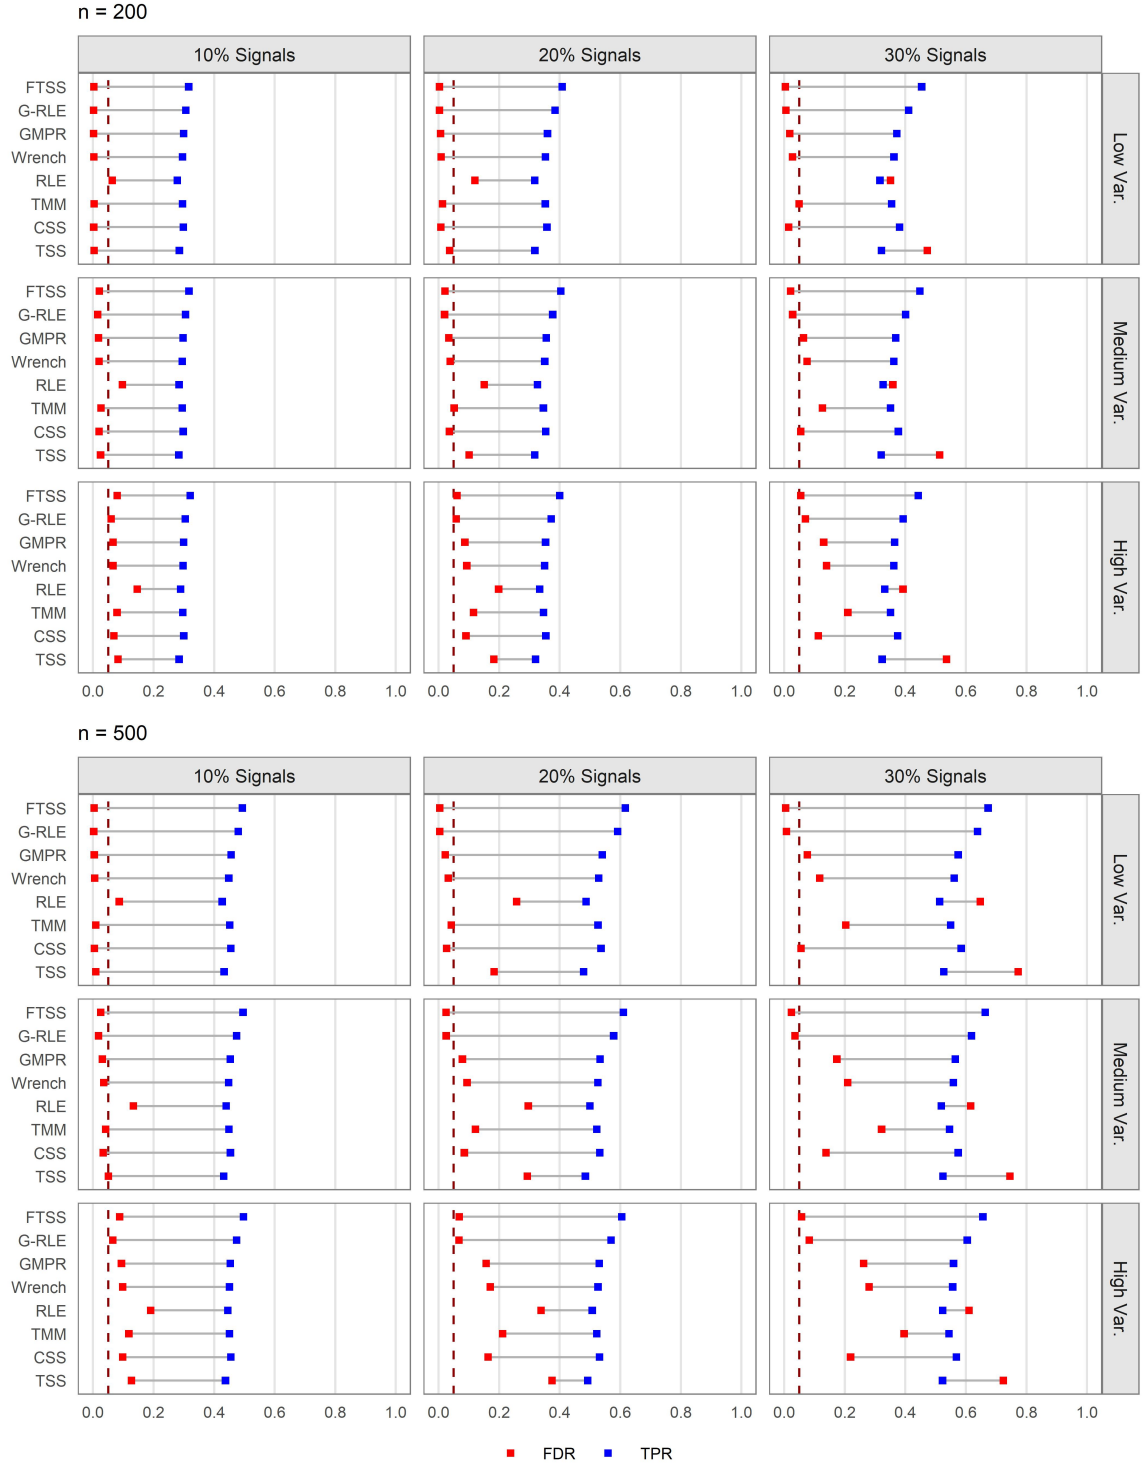

**Figure S8: Performance of normalization methods at nominal false discovery rate in model-based simulations with the DAA methods DESeq2.** The true positive rate (blue) and observed false discovery rate (red) corresponding to a nominal false discovery rate of 0.05 (the dashed line). Value shown is the mean over 1,000 replicates of each setting. The simulated datasets contain 300 taxa and either 200 or 500 samples. Either 10%, 20% or 30% of the taxa are differentially abundant, with log fold changes sampled from a Normal(1,1) distribution. Three different variance settings are considered.

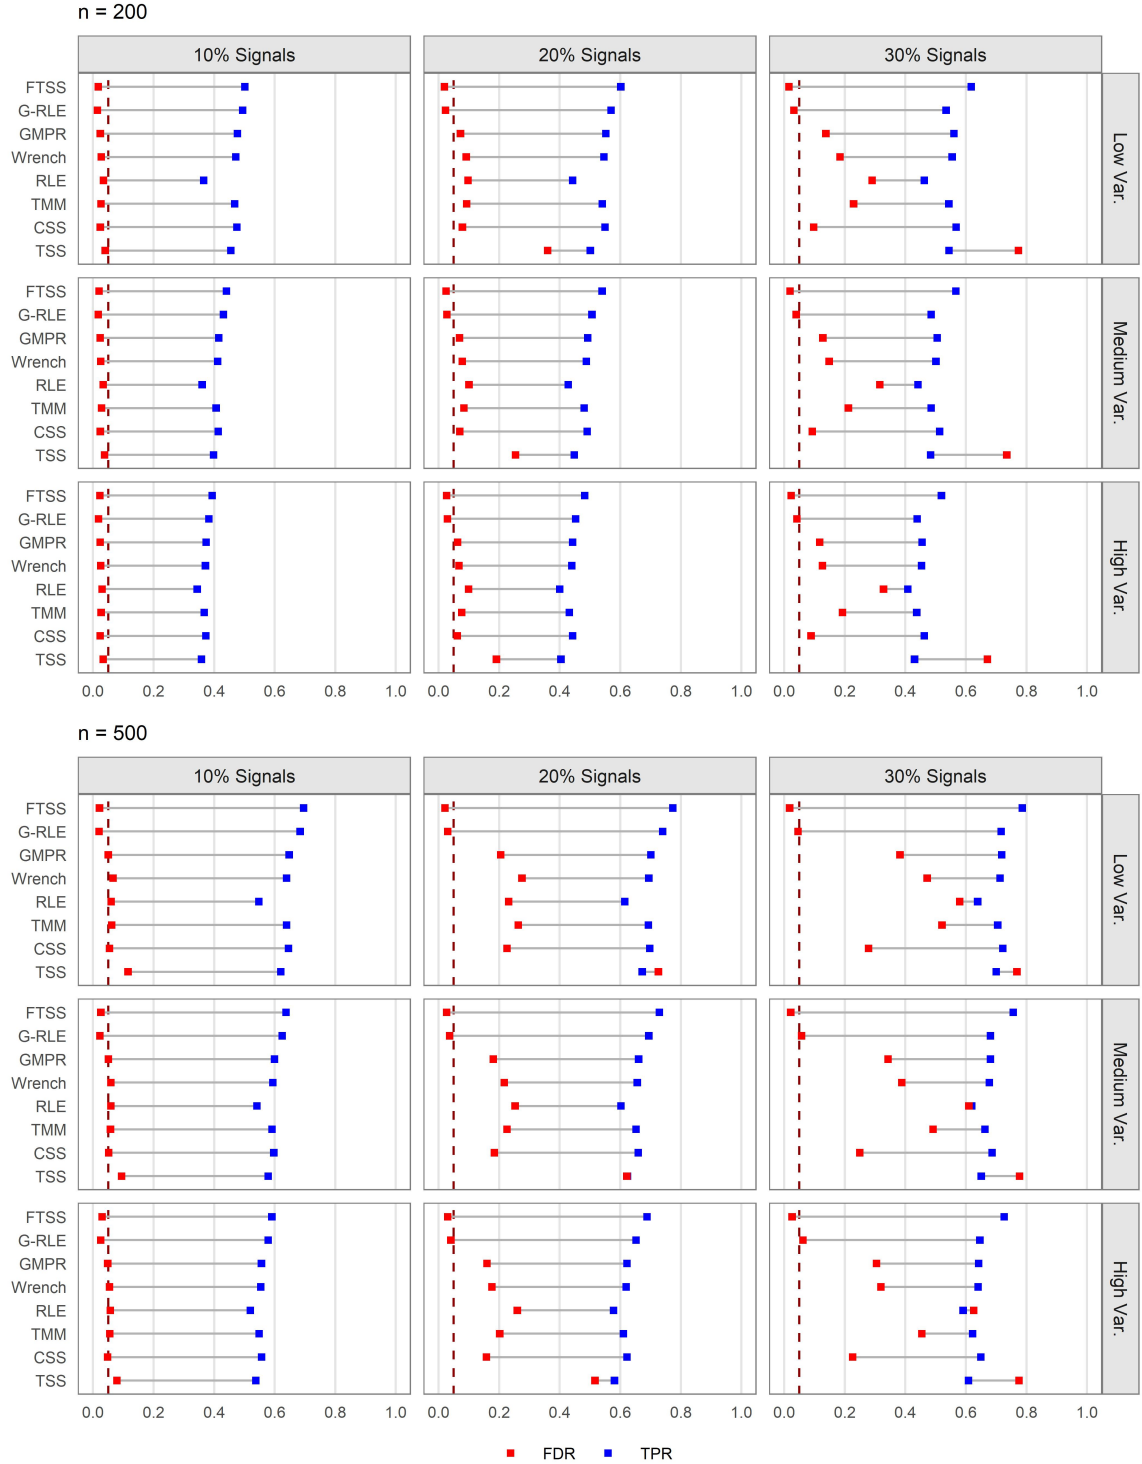

**Figure S9: Performance of normalization methods at nominal false discovery rate in model-based simulations with the DAA methods MetagenomeSeq.** The true positive rate (blue) and observed false discovery rate (red) corresponding to a nominal false discovery rate of 0.05 (the dashed line). Value shown is the mean over 1,000 replicates of each setting. The simulated datasets contain 300 taxa and either 200 or 500 samples. Either 10%, 20% or 30% of the taxa are differentially abundant, with log fold changes sampled from a  $\text{Normal}(1,1)$  distribution. Three different variance settings are considered.

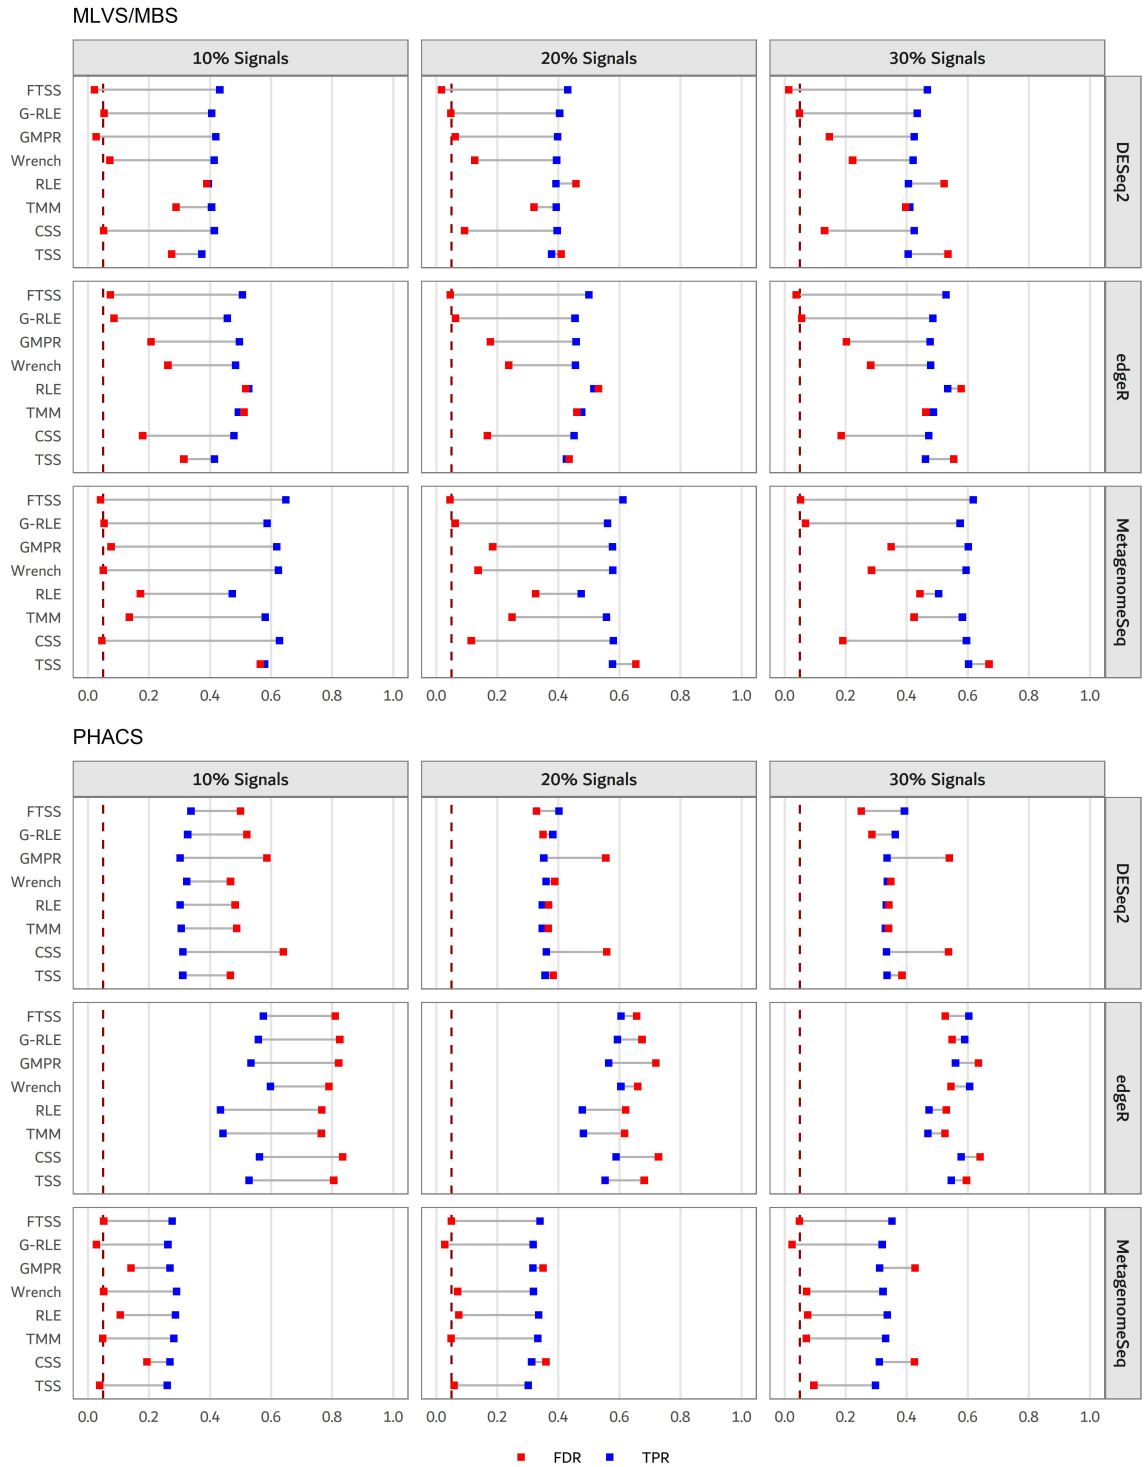

**Figure S10: Performance of normalization methods at nominal false discovery rate in synthetic data simulations.** The true positive rate (blue) and observed false discovery rate (red) corresponding to a nominal false discovery rate of 0.05 (the dashed line), for synthetic microbiome data based on either the MLVS/MBS or PHACS data. Value shown is the mean over 1,000 replicates of each setting. Either 10%, 20% or 30% of the taxa are differentially abundant, with log fold changes sampled from a  $\text{Normal}(1,1)$  distribution.

## References

- Michael I Love, Wolfgang Huber, and Simon Anders. Moderated estimation of fold change and dispersion for rna-seq data with *deseq2*. *Genome Biology*, 15(12):550, December 2014. ISSN 1474-760X. doi: 10.1186/s13059-014-0550-8.
- Joseph N Paulson, O Colin Stine, Héctor Corrada Bravo, and Mihai Pop. Differential abundance analysis for microbial marker-gene surveys. *Nature Methods*, 10(12):1200–1202, December 2013. ISSN 1548-7091, 1548-7105. doi: 10.1038/nmeth.2658.
- Mark D. Robinson, Davis J. McCarthy, and Gordon K. Smyth. *edgeR*: a bioconductor package for differential expression analysis of digital gene expression data. *Bioinformatics*, 26(1):139–140, January 2010. ISSN 1367-4811, 1367-4803. doi: 10.1093/bioinformatics/btp616.
